# Supplementary material for: Transcending Forgery Specificity with Latent Space Augmentation for Generalizable Deepfake Detection
Source: arXiv:2311.11278 source file (2024-03-28)
Supplement: Supplementary file 1 [file supp_ablation_WD.tex]

\begin{table*}
  \centering
  \scalebox{0.7}{
  \begin{tabular}{c|c|c|c|c|c|c} \toprule
    \multirow{2}*{Ablation} & DFD & CelebDF-v1 & CelebDF-v2 & DFDCP & DFDC & Avg.\\ 
    \cmidrule(lr){2-2}
    \cmidrule(lr){3-3}
    \cmidrule(lr){4-4}
    \cmidrule(lr){5-5}
    \cmidrule(lr){6-6}
    \cmidrule(lr){7-7}
    & AUC~$\uparrow$ ~\textbar~ AP~$\uparrow$ ~\textbar~ EER~$\downarrow$ & AUC~$\uparrow$ ~\textbar~ AP~$\uparrow$ ~\textbar~ EER~$\downarrow$ & AUC~$\uparrow$ ~\textbar~ AP~$\uparrow$ ~\textbar~ EER~$\downarrow$ & AUC~$\uparrow$ ~\textbar~ AP~$\uparrow$ ~\textbar~ EER~$\downarrow$ & AUC~$\uparrow$ ~\textbar~ AP~$\uparrow$ ~\textbar~ EER~$\downarrow$ & AUC~$\uparrow$ ~\textbar~ AP~$\uparrow$ ~\textbar~ EER~$\downarrow$ \\
    \midrule
    wo AdT & \textbf{0.884} ~\textbar~ \textbf{0.985} ~\textbar~ \textbf{19.8} & 0.860 ~\textbar~ 0.907 ~\textbar~ \textbf{21.7} & 0.824 ~\textbar~ 0.893 ~\textbar~ \textbf{25.7} & 0.800 ~\textbar~ 0.890 ~\textbar~ 27.3 & 0.740 ~\textbar~ \textbf{0.764} ~\textbar~ 32.7 & 0.814 ~\textbar~ 0.888 ~\textbar~ \textbf{25.4} \\
    wo AFT & 0.869 ~\textbar~ 0.982 ~\textbar~ 21.4 & 0.847 ~\textbar~ 0.904 ~\textbar~ 22.1 & 0.809 ~\textbar~ 0.884 ~\textbar~ 26.6 & \textbf{0.815} ~\textbar~ \textbf{0.898} ~\textbar~ \textbf{26.2} & \textbf{0.744} ~\textbar~ 0.762 ~\textbar~ \textbf{32.6} & 0.817 ~\textbar~ 0.886 ~\textbar~ 25.8 \\
    wo CT & 0.881 ~\textbar~ 0.984 ~\textbar~ 19.9 & 0.847 ~\textbar~ 0.898 ~\textbar~ 23.1 & 0.793 ~\textbar~ 0.877 ~\textbar~ 28.4 & 0.793 ~\textbar~ 0.878 ~\textbar~ 28.0 & 0.734 ~\textbar~ 0.756 ~\textbar~ 33.5 & 0.810 ~\textbar~ 0.879 ~\textbar~ 26.6 \\
    \midrule
    Ours & 0.880 ~\textbar~ 0.984 ~\textbar~ 20.0 & \textbf{0.867} ~\textbar~ \textbf{0.922} ~\textbar~ 21.9 & \textbf{0.830} ~\textbar~ \textbf{0.904} ~\textbar~ 25.9 & \textbf{0.815} ~\textbar~ 0.893 ~\textbar~ 26.9 & 0.736 ~\textbar~ 0.760 ~\textbar~ 33.0 & \textbf{0.825} ~\textbar~ \textbf{0.893} ~\textbar~ 25.5 \\
    \bottomrule
  \end{tabular}
  }
  \caption{
  Detailed performance metrics of different ablation studies. The values represent AUC, AP, and EER for each method across various datasets. The average performance (Avg.) across all datasets is also reported. The best results are highlighted in bold.
  }
  \label{tab:ablation_WD}
\end{table*}
